# Supplementary material for: Representation via Representations: Domain Generalization via Adversarially Learned Invariant Representations
Source: arXiv:2006.11478 source file (2020-06-20)
Supplement: Supplementary file 1 [file appendix_UD_comments.tex]

\newpage
\appendix
\noindent\textbf{\Large Supplementary Materials}
%===========================================
\section{Omitted Proofs}

\subsection{Proof of Theorem \ref{thm:limit} }
To begin with, we will establish that, under Assumption \ref{assumption:nds},
$$\lim_{k\rightarrow\infty}\sup_{\psi_k\in\Psi_k}\sum_{i=1}^{k}\bP_{x\sim\cD^\cX_i}(\pi_k\circ\psi_k(\phi(x))=i)\geq \sup_{\cup_iA_i=\bR^p,A_i\cap A_j=\emptyset, \zeta\in\Upsilon}\sum_{i=1}^{N}\bP_{x\sim\cD^{*\cX}_i}(\zeta(\phi(x))\in A_i)$$
This is achieved using a geometric argument. We proceed by considering simple settings first, before moving on to the most general case.
\paragraph{Step 1.} Consider the case of $p=1$. For fixed $\phi$ and $\zeta$, for any $\varepsilon>0$, one can choose a constant $C_\varepsilon>0$, such that 
\begin{equation}\label{eq:tailcontrol}
\sum_{i=1}^{N}\bP_{x\sim \cD^{*\cX}_i}(|\varphi(\phi(x))|\geq C_\varepsilon)\leq \varepsilon.
\end{equation}
Now, when $k$ is very large, say  $k\gg N$, we would expect that every $\cD^{*\cX}_i$'s shows up at least $n_k$ times with high probability $1-\delta_k$ for some $n_k$ and $\delta_k$. Since $\mu$ assigns a positive probability  to each domain $\cD^{*\cX}_i$ and $N$ is finite, we can have a universal lower bound for the $p_i$'s. Then, by standard arguments, one can choose $n_k$ and $\delta_k$ such that when $k\rightarrow\infty$, we have $n_k\rightarrow\infty$ and $\delta_k\rightarrow 0$. {\color{red}PS: I would fill in the arguments for the arxiv version. }

For such a sequence of  $n_k$'s,  the interval $[-C_\varepsilon,C_\varepsilon]$ can subdivided into a collection of $n_k$ intervals $\cS=\{I_1,I_2,\cdots, I_{n_k}\}=\{[-C_\varepsilon,-C_\varepsilon+2C_\varepsilon/n_k],[- C_\varepsilon+2C_\varepsilon/n_k,-C_\varepsilon+4C_\varepsilon/n_k] ,\cdots,[C_\varepsilon-2C_\varepsilon/n_k,C_\varepsilon]\}$, such that the intersection of each pair has $0$ measure in $1$-dimensional space.

Next, we establish that, if each $\cD^{*\cX}_i$ shows up with at least $n_k$ times, we have
\begin{equation}\label{eq:inq}
\sup_{\psi_k\in\Psi_k}\sum_{i=1}^{k}\bP_{x\sim\cD^\cX_i}(\pi_k\circ\psi_k(\phi(x))=i)\geq \sup_{A_i\subseteq \cS, \cup_iA_i=\cS,A_i\cap A_j=\emptyset, \zeta\in\Upsilon}\sum_{i=1}^{N}\bP_{x\sim\cD^{*\cX}_i}(\zeta(\phi(x))\in A_i).
\end{equation}

To this end, define
$$\cD^{*\cX}_{I_i}=  \argmax_{\cD^{*\cX}_l} \bP_{x\sim\cD^{*\cX}_l}(\zeta(\phi(x))\in I_i)$$
%{\color{red} I am not sure if this was great notation, if needs change will defer to arxiv version.}
Whenever there are multiple maximizers, we randomly pick one of them. {\color{red} PS: Why would this process not stop in between?}
{\color{red} (notice that this will not affect value of the RHS in Eq.\ref{eq:inq})}. {\color{red} PS: Unsure what this comment tries to say. } Now, recall that
$$\psi_k(\cdot)=W\zeta(\cdot) +B.$$ 
For $\cD^{*\cX}_{I_i}$, we denote the corresponding parameters of the linear transformation by $w_{I_i}$, $b_{I_i}$ .  Choose
$$w_{I_1}=\frac{\pi }{2(n_k+1)}, b_{I_1}=C_\varepsilon w_{I_1};$$
$$w_{I_i}=\frac{\pi i}{2(n_k+1)}, b_{I_i}=(w_{I_{i-1}}-w_{I_{i}})(-C_\varepsilon+\frac{2C_\varepsilon(i-1)}{n_k})+b_{I_{i-1}}.~~i\geq 2.$$
For the remaining entries of $W, B$ simply let $w_i=0, b_i=0$. As a consequence, $w_{I_i}z+b_{I_i}$ will be the largest when $z\in I_i$, where $z=\zeta(\phi(x))$ (the intersections are of measure $0$, so we simply  ignore them).  If $E$ is the event that ``all $\cD^{*\cX}_i$ appears more than $n_k$ times'', we have with probability at least $\bP(E)$ that
$$\sup_{\psi_k\in\Psi_k}\sum_{i=1}^{k}\bP_{x\sim\cD^\cX_i}(\pi_k\circ\psi_k(\phi(x))=i)\geq \sup_{A_i\subseteq \cS, \cup_iA_i=\cS,A_i\cap A_j=\emptyset, \zeta\in\Upsilon}\sum_{i=1}^{N}\bP_{x\sim\cD^{*\cX}_i}(\zeta(\phi(x))\in A_i )-\varepsilon.$$
where $E$ is the event ``all $\cD^{*\cX}_i$ appears more than $n_k$ times''. Since  $n_k\rightarrow \infty$, $\delta_k\rightarrow 0$, we have as $k\rightarrow\infty$, with probability $1$, {\color{red} It is crucial to make this jump, what $\delta_k$ is since this seems like a Borel-Cantelli argument. Need to include details for arxiv version.}
$$\lim_{k\rightarrow\infty}\sup_{\psi_k\in\Psi_k}\sum_{i=1}^{k}\bP_{x\sim\cD^\cX_i}(\pi_k\circ\psi_k(\phi(x))=i)\geq \sup_{\cup_iA_i=\bR^p,A_i\cap A_j=\emptyset, \zeta\in\Upsilon}\sum_{i=1}^{N}\bP_{x\sim\cD^{*\cX}_i}(\zeta(\phi(x))\in A_i\cap[-C_\varepsilon,C_\varepsilon])-\varepsilon.$$
This is true because Assumption \ref{assumption:nds} implies that each region $T^{\zeta,\phi}_i$ (see main article for definition) can be approximated to an arbitrary degree by small enough intervals. {\color{red}PS: This is an analytic argument that needs details for arxiv version. } Notice $\varepsilon$ can be arbitrarily small, thus, we have 

$$\lim_{k\rightarrow\infty}\sup_{\psi_k\in\Psi_k}\sum_{i=1}^{k}\bP_{x\sim\cD^\cX_i}(\pi_k\circ\psi_k(\phi(x))=i)\geq \sup_{\cup_iA_i=\bR^p,A_i\cap A_j=\emptyset, \zeta\in\Upsilon}\sum_{i=1}^{N}\bP_{x\sim\cD^{*\cX}_i}(\zeta(\phi(x))\in A_i).$$

%====================
\paragraph{Step 2.} Now let us consider $p=2$. Here as well \eqref{eq:tailcontrol} continues to hold. 
%Again we can choose a constant $C_\varepsilon>0$, such that 
%$$\sum_{i=1}^{N}\bP_{x\sim \cD^{*\cX}_i}(\|\varphi(\phi(x))\|_\infty\geq C_\varepsilon)\leq \varepsilon.$$
When $k$ is very large so that $k\gg N$, we would expect that each $\cD^{*\cX}_i$ shows up at least $n^2_k$ times with high probability $1-\delta_k$ for some $n_k$ and $\delta_k$. Now, subdivide the square  $[-C_\varepsilon,C_\varepsilon]\times [-C_\varepsilon,C_\varepsilon]$, into smaller chunks   $\{I_{ij}\}$ such that $I_{i,j}=[-C_\varepsilon+2(i-1)C_\varepsilon/n_k, -C_\varepsilon+2iC_\varepsilon/n_k]\times [-C_\varepsilon+2(j-1)C_\varepsilon/n_k, -C_\varepsilon+2jC_\varepsilon/n_k]$.

Again, let $z=(z_1,z_2)\in\bR^2$ denote $\zeta(\phi(x))$. Each node in the last layer of the linear transformation has the following form:
$$w^\top z +b=w_1^\top z_1+w_2^\top z_2 +b$$
In this case, define
$$\cD^{*\cX}_{I_{ij}}= \argmax_{\cD^{*\cX}_l} \bP_{x\sim\cD^{*\cX}_l}(\varphi(\phi(x))\in I_{ij})$$
If there are multiple maximizers, we pick one of them at random.  For $\cD^{*\cX}_{I_{i,j}}$, we denote the corresponding parameters of the linear transformation as $w_{1,I_{i,j}}$, $w_{2,I_{i,j}}$ and $b_{I_{i,j}}$. For $j=1$, let 
$$w_{1, I_{1,1}}=\frac{\pi }{2(n_k+1)}, w_{2, I_{1,1}}=0, b_{I_{1,1}}=C_\varepsilon w_{1,I_{1,1}};$$
$$w_{1,I_{i,1}}=\frac{\pi i}{2(n_k+1)}, b_{I_{i,1}}=(w_{1,I_{i-1,1}}-w_{1,I_{1,i}})(-C_\varepsilon+\frac{2C_\varepsilon(i-1)}{n_k})+b_{I_{i-1,1}}.~~i\geq 2.$$

For $j>1$, we choose parameters so that $w_{I_{i,j}}^\top z+b_{I_{i,j}}=w_{I_{i,j-1}}^\top z+b_{I_{i,j-1}}$ whenever $z\in [-C_\varepsilon+2(i-1)C_\varepsilon/n_k, -C_\varepsilon+2iC_\varepsilon/n_k]\times\{-C_\varepsilon+2(j-1)C_\varepsilon/n_k\}.$ Meanwhile, for all $i,j$, we let 
$$w_{2,I_{i,j}}=\frac{j\pi }{2(n_k+1)},w_{1,I_{i,j}}=w_{1,I_{i,j-1}}$$
Then, we can obtain 
$$b_{I_{i,j}}=b_{I_{i,j-1}}-\frac{\pi }{2(n_k+1)}(-C_\varepsilon+2(j-1)C_\varepsilon/n_k).$$
Once again, for the remaining parameters, let $w_i=0, b_i=0$ and this leads to $w_{I_{i,j}}z+b_{I_{i,j}}$ being the largest when $z\in I_{i,j}$. Using a similar argument as in step 1, we then have 
\begin{equation*}
\sup_{\psi_k\in\Psi_k}\sum_{i=1}^{k}\bP_{x\sim\cD^\cX_i}(\pi_k\circ\psi_k(\phi(x))=i)\geq \sup_{A_{i}\subseteq \cS, \cup_iA_{i}=\cS,A_{i}\cap A_{j}=\emptyset, \zeta\in\Upsilon}\sum_{i=1}^{N}\bP_{x\sim\cD^{*\cX}_i}(\zeta(\phi(x))\in A_{i}),
\end{equation*}
where $\cS=\{I_{i,j}\}_{i,j}$.
%====================
\paragraph{Step 3.} For $p>2$, we can similarly use $p$-dimensional cubes $I_{i_1,i_2,\cdots,i_p}$ to divide a bounded cube with length of edges equal to some constant $C_\varepsilon$. When we have assigned values to $\{w_{j,I_{i_1,\cdots,i_p}}\}_{j=1,\cdots,n_k}$ and $b_{I_{i_1,\cdots,p}}$, we can use induction to sequentially assign values to $w_{p,I_{i_1,\cdots,i_p}}$ and $\{b_{I_{i_1,\cdots,j}}\}_{j\geq 2}$, such that 
$$w_{I_{i_1,i_2,\cdots,j}}^\top z+b_{I_{i_1,i_2,\cdots,j}}=w_{I_{i_1,i_2,\cdots,j-1}}^\top z+b_{I_{i_1,i_2,\cdots,j-1}}$$
on the $p-1$ dimensional segment $z\in I_{i_1,\cdots,i_{p-1}}\times\{-C_\varepsilon+2(j-1)C_\varepsilon/n_k\}$ and $w_{k,I_{i_1,\cdots,j}}:=j\pi/2(n_k+1)$. This finally leads to
\begin{equation*}
\lim_{k\rightarrow \infty}\sup_{\psi_k\in\Psi_k}\sum_{i=1}^{k}\bP_{x\sim\cD^\cX_i}(\pi_k\circ\psi_k(\phi(x))=i)\geq\sup_{\cup_iA_i=\bR^p,A_i\cap A_j=\emptyset, \zeta\in\Upsilon}\sum_{i=1}^{N}\bP_{x\sim\cD^\cX_i}(\zeta(\phi(x))\in A_i).
\end{equation*}

\paragraph{Step 4.}It remains to show the other direction, i.e.
\begin{equation*}
\lim_{k\rightarrow \infty}\sup_{\psi_k\in\Psi_k}\sum_{i=1}^{k}\bP_{x\sim\cD^\cX_i}(\pi_k\circ\psi_k(\phi(x))=i)\leq\sup_{\cup_iA_i=\bR^p,A_i\cap A_j=\emptyset, \zeta\in\Upsilon}\sum_{i=1}^{N}\bP_{x\sim\cD^\cX_i}(\zeta(\phi(x))\in A_i).
\end{equation*}
We first show that for 
$$\tilde{\psi}_k\in\argmax_{\psi_k\in\Psi_k}\sum_{i=1}^{k}\bP_{x\sim\cD^\cX_i}(\pi_k\circ\psi_k(\phi(x))=i),$$
(we use $\in$ here since there may be multiple maximizers), WLOG, we can assume the corresponding $(\tilde{w}_i,\tilde{b}_i)$'s are all distinct, i.e. for any $i\neq j$ $(\tilde{w}_i,\tilde{b}_i)\neq (\tilde{w}_j,\tilde{b}_j)$. For simplicity, for two (and only two) domains $\cD_i$ and $\cD_j$, if $(\tilde{w}_i,\tilde{b}_i)= (\tilde{w}_j,\tilde{b}_j)$ and if we pick randomly in the presence of ties, then
$$\bP_{x\sim\cD^\cX_i}(\pi_k\circ\tilde{\psi}_k(\phi(x))=i)+\bP_{x\sim\cD^\cX_j}(\pi_k\circ\tilde{\psi}_k(\phi(x))=j)\leq \max\{\bP_{x\sim\cD^\cX_i}(\tilde{\zeta}(\phi(x))\in T) ,\bP_{x\sim\cD^\cX_j}(\tilde{\zeta}(\phi(x))\in T)\},$$
where $T=\{z:\tilde{w}_i^\top z+\tilde{b}_i>\tilde{w}_l^\top z+\tilde{b}_l~\text{for}~l\neq i,j\}$. If $\bP_{x\sim\cD^\cX_i}(\tilde{\zeta}(\phi(x))\in T) >\bP_{x\sim\cD^\cX_j}(\tilde{\zeta}(\phi(x))\in T) $, we can simply reassign the $j$-th node's weights to $w'_j,b'_j$ such that ${w'_j}^\top z+b'_j<\min_{l\neq j}\tilde{w}_l^\top z+\tilde{b}_l$ for all $z$, but without decreasing the value of $\sup_{\psi_k\in\Psi_k}\sum_{i=1}^{k}\bP_{x\sim\cD^\cX_i}(\pi_k\circ\psi_k(\phi(x))=i)$. So, there must exist a maximizer $\tilde{\psi}_k$ such that for any $i\neq j$ $(\tilde{w}_i,\tilde{b}_i)\neq (\tilde{w}_j,\tilde{b}_j)$. Meanwhile if  $i\neq j$ $(\tilde{w}_i,\tilde{b}_i)\neq (\tilde{w}_j,\tilde{b}_j)$, then $\{z: \exists i\neq j,~s.t.~\tilde{w}_i^\top z+\tilde{b}_i=\tilde{w}_j^\top z+\tilde{b}_j\}$ is of measure $0$ in $\bR^p$ since $\mathrm{Supp}_{\zeta(\phi(\cD^{*\cX}_i))}$ has non-zero volume in $\mathbb{R}^p$ and  the collection of $z$ such that
$$(\tilde{w}_i-\tilde{w}_j)^\top z=\tilde{b}_j-\tilde{b}_i$$
has volume $0$ in $\bR^p$.

Consequently, we can divide $\bR^p$ into disjoint regions  $T_i=\{z:\tilde{w}_i^\top z+\tilde{b}_i>\tilde{w}_l^\top z+\tilde{b}_l~\text{for}~l\neq i\}$, and
\begin{align*}
\sup_{\psi_k\in\Psi_k}\sum_{i=1}^{k}\bP_{x\sim\cD^\cX_i}(\pi_k\circ\psi_k(\phi(x))=i) & =\sum_{i=1}^{k}\bP_{x\sim\cD^\cX_i}(\tilde{\zeta}(\phi(x))\in T_i) \\
& \leq \sup_{\cup_iA_i=\bR^p,A_i\cap A_j=\emptyset, \zeta\in\Upsilon}\sum_{i=1}^{N}\bP_{x\sim\cD^\cX_i}(\zeta(\phi(x))\in A_i).
\end{align*}
Then letting $k\rightarrow\infty$ completes the proof.
%=========================================
\subsection{Proof of Theorem \ref{thm:non-asymptotic bound}}
We proceed with several lemmas.

\begin{lemma}\label{lm:s1}
With probability at least $1-\exp(-k^{1/4})$ over the randomness of $\{\cD^{\cX}_i\}_{i=1}^{k}$, for all $\zeta\in\Upsilon$ and $\phi\in\Phi$
\begin{align*}
&|\sup_{\cup_iA_i=\bR^p,A_i\cap A_j=\emptyset}\sum_{i\in H_k}\bP_{x\sim\cD^{*\cX}_i}(\zeta(\phi(x))\in A_i)-\sum_{i\in H_k}\bP_{x\sim\cD^{*\cX}_i}(\zeta(\phi(x))\in M^{\zeta,\phi}_{i,2}(\lfloor m^{1/p}_k \rfloor,B(\frac{1}{\sqrt{k}})))| \\
&\leq\frac{2B_\rho \left(B(\frac{1}{\sqrt{k}})\right)^{p}}{\lfloor m^{1/p}_k \rfloor^p } \sum_{i\in H_k}\sup_{\zeta,\phi}|M^{\zeta,\phi}_{i,1}(\lfloor m^{1/p}_k \rfloor,B(\frac{1}{\sqrt{k}}))|+\frac{1}{\sqrt{k}}.
\end{align*}
\end{lemma}
\begin{proof}
Recall that we defined $H_k$ to be the set of domains that receive $\mu$-probability larger than or equal to $p^*_k=1/k^{1/4}$. Note that the probability that all domains in $H_k$ have been observed at least $m_k$ times is lower bounded by 
$$1-|H_k|\cdot\sum_{i=0}^{m_k}C^{i}_kp_k^{*i}(1-p^*_k)^{k-i},$$
which is further lower bounded, via Hoeffding's inequality, by
$$\beta=1-|H_k|\cdot\exp(-2\frac{(kp^*_k-m_k)^2}{k}).$$
If we choose $m_k =\lceil k^{\frac{3}{4}}-\sqrt{(k\log(|H_k|)+k^{\frac{3}{4}})/ \sqrt{2}}\rceil$, then
$$\beta\geq 1-\exp(-k^{1/4}).$$
From our assumptions, it follows that $\sup_{\zeta,\phi}\sum_{i=1}^{N}\bP_{x\sim \cD^{*\cX}_i}(\|\zeta(\phi(x))\|_2\geq B(1/\sqrt{k}))\leq 1/\sqrt{k}$. 
%We treat the probability $1/\sqrt{k}$ as error term. 
Then, we can operate on the cube $[-B(1/\sqrt{k}),B(1/\sqrt{k})]^{\times p}$ and divide it into $\lfloor m^{1/p}_k\rfloor^p$ small cubes of volume $(B(1/\sqrt{k}))^p/\lfloor m^{1/p}_k\rfloor^p$ each, as in the proof of Theorem \ref{thm:limit}. Since all the elements in $H_k$ will show up at least $m_k$ times, we can then assign weights in a manner similar to that  in Theorem \ref{thm:limit}. Recall  that $\sup_{z,\zeta,\phi,i}|\rho^{\zeta,\phi}_i(z)|\leq B_\rho$, which completes the proof.
\end{proof}

The following is a direct corollary of Lemma \ref{lm:s1}.
\begin{corollary}\label{lemma:s2}
With probability at least $1-\exp(-k^{1/4})$ over the randomness of $\{\cD^{\cX}_i\}_{i=0}^{k-1}$
\begin{align*}
&\sup_{\zeta,\phi}|\sup_{\cup_iA_i=\bR^p,A_i\cap A_j=\emptyset}\sum_{i=1}^{N}\bP_{x\sim\cD^{*\cX}_i}(\zeta(\phi(x))\in A_i)-\sup_{\cup_iA_i=\bR^p,A_i\cap A_j=\emptyset}\sum_{i\in H_k}\bP_{x\sim\cD^{*\cX}_i}(\zeta(\phi(x))\in A_i)
|\\
&\leq\frac{2B_\rho \left(B(\frac{1}{\sqrt{k}})\right)^{p}}{\lfloor m^{1/p}_k \rfloor^p } \sum_{i\in H_k}\sup_{\zeta,\phi}|M^{\zeta,\phi}_{i,1}(\lfloor m^{1/p}_k \rfloor,B(\frac{1}{\sqrt{k}}))|+\frac{1}{\sqrt{k}}+\max\{N-|H_k|,0\}.
\end{align*}
\end{corollary}
\begin{proof}
For any $\tilde{\zeta}\in\argmax_{\zeta\in\Upsilon}\sup_{\cup_iA_i=\bR^p,A_i\cap A_j=\emptyset}\sum_{i=1}^{N}\bP_{x\sim\cD^{*\cX}_i}(\zeta(\phi(x))\in A_i) $, we know that
\begin{align*}
\sup_{\cup_iA_i=\bR^p,A_i\cap A_j=\emptyset}\sum_{i=1}^{N}\bP_{x\sim\cD^{*\cX}_i}(\tilde{\zeta}(\phi(x))\in A_i)&\geq \sup_{\cup_iA_i=\bR^p,A_i\cap A_j=\emptyset, \zeta\in\Upsilon}\sum_{i\in H_k}\bP_{x\sim\cD^{*\cX}_i}(\zeta(\phi(x))\in A_i)\\
&\geq \sup_{\cup_iA_i=\bR^p,A_i\cap A_j=\emptyset}\sum_{i\in H_k}\bP_{x\sim\cD^{*\cX}_i}(\tilde{\zeta}(\phi(x))\in A_i).
\end{align*}
Then, the results follows immediately by noticing that a probability is always bounded by 1.

\end{proof}

Besides, we can easily see that with probability at least $1-\exp(-k^{1/4})$ over the randomness of $\{\cD^{\cX}_i\}_{i=1}^{k}$
\begin{align*}
\sup_{\psi_k\in\Psi_k}\sum_{i=1}^{k}\bP_{x\sim\cD^\cX_i}(\pi_k\circ\psi_k(\phi(x))=i)&\geq\sup_{\psi_k\in\Psi_k}\sum_{i\in H_k}\bP_{x\sim\cD^\cX_i}(\pi_{H_k}\circ\psi_{H_k}(\phi(x))=i)\\&\geq\sup_{\zeta\in\Upsilon}\sum_{i\in H_k}\bP_{x\sim\cD^{*\cX}_i}(\zeta(\phi(x))\in M^{\zeta,\phi}_{i,2}(\lfloor m^{1/p}_k \rfloor,B(\frac{1}{\sqrt{k}}))).
\end{align*}

Also, we have that
\begin{equation*}
\sup_{\psi_k\in\Psi_k}\sum_{i\in H_k}\bP_{x\sim\cD^\cX_i}(\pi_{H_k}\circ\psi_{H_k}(\phi(x))=i)\leq\sup_{\cup_iA_i=\bR^p,A_i\cap A_j=\emptyset, \zeta\in\Upsilon}\sum_{i\in H_k}\bP_{x\sim\cD^\cX_i}(\zeta(\phi(x))\in A_i),
\end{equation*}

\begin{equation*}
\sup_{\psi_k\in\Psi_k}\sum_{i=1}^N\bP_{x\sim\cD^\cX_i}(\pi_{N}\circ\psi_{N}(\phi(x))=i)\leq\sup_{\cup_iA_i=\bR^p,A_i\cap A_j=\emptyset, \zeta\in\Upsilon}\sum_{i=1}^N\bP_{x\sim\cD^\cX_i}(\zeta(\phi(x))\in A_i).
\end{equation*}
Now, 
\begin{align*}
&|\sup_{\cup_iA_i=\bR^p,A_i\cap A_j=\emptyset, \zeta\in\Upsilon}\sum_{i=1}^N\bP_{x\sim\cD^\cX_i}(\zeta(\phi(x))\in A_i)-\sup_{\cup_iA_i=\bR^p,A_i\cap A_j=\emptyset, \zeta\in\Upsilon}\sum_{i\in H_k}\bP_{x\sim\cD^\cX_i}(\zeta(\phi(x))\in A_i)|\\
&\leq \max\{N-|H_k|,0\}
\end{align*}
by Corollary \ref{lemma:s2} and similarly 
$$|\max_{\psi_{H_k}\in\Psi_{H_k}}\sum_{i\in H_k}\bP_{x\sim\cD^\cX_i}(\pi_{H_k}\circ\psi_{H_k}(\phi(x))=i)-\max_{\psi_N\in\Psi_N}\sum_{i=1}^{N}\bP_{x\sim\cD^\cX_i}(\pi_N\circ\psi_N(\phi(x))=i)|\leq \max\{N-|H_k|,0\},$$
$$\max_{\psi_k\in\Psi_k}\sum_{i=1}^{k}\bP_{x\sim\cD^\cX_i}(\pi_k\circ\psi_k(\phi(x))=i)\leq \max_{\psi_N\in\Psi_N}\sum_{i=1}^{N}\bP_{x\sim\cD^\cX_i}(\pi_N\circ\psi_N(\phi(x))=i).$$
Together these lead to the following lemma.  
\begin{lemma}\label{lemma:s3}
\begin{align*}
&|\max_{\psi_k\in\Psi_k}\sum_{i=1}^{k}\bP_{x\sim\cD^\cX_i}(\pi_k\circ\psi_k(\phi(x))=i)-\sup_{\cup_iA_i=\bR^p,A_i\cap A_j=\emptyset, \zeta\in\Upsilon}\sum_{i=1}^{N}\bP_{x\sim\cD^{*\cX}_i}(\zeta(\phi(x))\in A_i)|\\
&\leq \frac{2B_\rho \left(B(\frac{1}{\sqrt{k}})\right)^{p}}{\lfloor m^{1/p}_k \rfloor^p } \sum_{i\in H_k}\sup_{\zeta,\phi}|M^{\zeta,\phi}_{i,1}(\lfloor m^{1/p}_k \rfloor,B(\frac{1}{\sqrt{k}}))|+\frac{1}{\sqrt{k}}+\max\{N-|H_k|,0\}.
\end{align*}
\end{lemma}

Furthermore, by traditional VC-dimension argument, we have the following. 
\begin{lemma}
Under Assumption \ref{assumption:vc}, there exists a universal constant $c>0$ such that for any $t>0$, with probability at least $1-2e^{-n_it^2}$, 
$$|\frac{1}{k}\sum_{i=1}^k\bP_{(x,y)\sim\cD_i}(f(\phi(x))\neq y)- \frac{1}{k}\sum_{i=1}^{k}\frac{1}{n_i}\sum_{j=1}^{n_i}\mI\{f(\phi(x_{i,j}))\neq y_{i,j}\}|\leq t+c\sqrt{\frac{\cV_\Lambda\log(n_i/\cV_\Lambda)}{n_i}} .$$
\end{lemma}

\begin{lemma}
Under Assumption \ref{assumption:vc}, there exists a universal constant $c>0$ such that for any $t>0$, with probability at least $1-2e^{-n_it_1^2}-2N\exp(-2kt_2^2)$, 
$$|\bE_{\cD\sim\mu}\bP_{(x,y)\sim\cD}(f(\phi(x))\neq y)- \frac{1}{k}\sum_{i=1}^{k}\frac{1}{n_i}\sum_{j=1}^{n_i}\mI\{f(\phi(x_{i,j}))\neq y_{i,j}\}|\leq t_1+c\sqrt{\frac{\cV_\Lambda\log(n_i/\cV_\Lambda)}{n_i}}+Nt_2 $$
\end{lemma}

\begin{proof}
By Hoeffding inequality, and the fact that 
$$|\frac{1}{k}\sum_{i=1}^{k}\bP_{(x,y)\sim\cD_i}(f(\phi(x))\neq y)-\bE_{
\cD\sim \mu}[\bP_{(x,y)\sim\cD}(f(\phi(x))\neq y)|\leq \sum_{i=1}^{N}|\hat {p}_i-p_i |,$$
where $p_i$ is the mass of $\cD^{*}_i$ and $\hat{p}_i$ is the corresponding empirical mass induced by the observed samples, we know, with probability at least $1-2N\exp(-2kt_2^2)$, 
$$\sup_{f,\phi}|\frac{1}{k}\sum_{i=1}^{k}\bP_{(x,y)\sim\cD_i}(f(\phi(x))\neq y)-\bE_{
\cD\sim \sD}[\bP_{(x,y)\sim\cD}(f(\phi(x))\neq y)|\leq Nt_2.$$

\end{proof}

%=============
%==========
\begin{lemma}\label{lm:vc}
Under Assumptions \ref{assumption:nds} and \ref{assumption:vc},  if $\tilde{\Psi}_k\subseteq\Psi_k$ is such that the last layer satisfies $ (w_i,b_i)\neq (w_j,b_j)$ whenever $i\neq j$, then there exists a universal constant $c>0$ so that for any $t>0$, with probability at least $1-2e^{-n_it^2}$,
\begin{align*}
\sup_{\psi_k\in\tilde{\Psi}_k,\phi\in\Phi}&|\frac{1}{n_i}\sum_{j=1}^{n_i}( \mI\{\pi_k\circ\psi_{k}(\phi(x_{i,j}))=i\}-\bP_{x\sim\cD^\cX_i}(\pi_k\circ\psi(\phi(x)))=i)|\leq t+c\sqrt{\frac{\cV_{C(k)}\log(n_i/\cV_{C(k)})}{n_i}}\end{align*}
\end{lemma}
\begin{proof}
Note that $\{x:\pi_2\circ \tilde{\psi}_2(x)=1\}=\{x:w_1^\top\tilde{\zeta}(x)+b_1>w_2^\top\tilde{\zeta}(x)+b_2\}$ up to a set of measure $0$ for the corresponding $\tilde{\zeta}$, under the continuity assumption. In fact, if we consider our setting which has $k$ classes, then once again, $\{x:\pi_k\circ \tilde{\psi}_k(x)=i\}=\{x:w_i^\top\tilde{\zeta}(x)+b_i>\max_{j\neq i}w_j^\top\tilde{\zeta}(x)+b_j\}$ up to a set of measure $0$.

\begin{align*}
\cC(k)&=\{\mI\{\max_{j\neq i}w_j^\top\zeta(\phi(x))\leq w_i^\top\zeta(\phi(x))\}|w_1,\cdots,w_{k}\in\bR^p,\zeta\in\Upsilon,\phi\in\Phi\}\\
&=\{\Pi_{j\neq i}\bI\{w_j^\top\zeta(\phi(x))\leq w_i^\top\zeta(\phi(x))\}|w_1,\cdots,w_{k}\in\bR^p,\zeta\in\Upsilon,\phi\in\Phi\}.
\end{align*}
By Sauer-Shelah Lemma, we know that for an $m$ element set, $\cC(k)$ can pick up at most $O(m^{k\cV_{\Xi}})$ distinct subsets. Thus, as long as
$$2^m\geq c \cdot m^{k\cV_{\Xi}}$$ 
for some universal constant $c$, then the VC-dimension of $\cC(k)\leq m$. We know that for large $k$, $m=O(k\cV_{\Xi}(\log(\cV_{\Xi}))^2)$,
since
$$\mI\{\mI\{\max_{j\neq i}w_j^\top\zeta(\phi(x))+b_j< w_i^\top\zeta(\phi(x))+b_i\}\neq 0\}=\mI\{\max_{j\neq i}w_j^\top\varphi(\phi(x))< w_i^\top\varphi(\phi(x))\}.$$
Then applying traditional uniform convergence theories on samples $\{(x_{i,j},0)\}_{j=1}^{n_i}$ and distributions $(\cD^{\cX}_i,0)$, the result follows. 
\end{proof}

As we discussed in Theorem \ref{thm:limit}, one of the maximizers must belong to $\tilde{\Psi}_k$. Combining everyhting and using similar squeezing argument as in Theorem  \ref{thm:limit}, completes the proof of Theorem \ref{thm:non-asymptotic bound}.

%=========================================
\subsection{Example for Theorem \ref{thm:non-asymptotic bound}}
We give a specific example here to illustrate the bound: consider that there are only $2$ elements in $\sD$, $p=2$ and 
$$T_1=\{(x_1,x_2): x_1\leq c \}$$
for a constant $c$. Then we know that
$$\sum_{i\in H_k}\sup_{\zeta,\phi}|M^{\zeta,\phi}_{i,1}(\lfloor m^{1/p}_k \rfloor,B(\frac{1}{\sqrt{k}}))|=O(\lfloor m^{1/2}_k \rfloor)$$
If we further suppose that all the distributions in $\sD$of  are multivariate sub-gaussian , with sub-gaussian norm all bounded by a constant $\sigma_{\max}$, then 
$$B(\frac{1}{\sqrt{k}})=O(\sqrt{\log k}).$$
Thus , we have 
$$\frac{B_\rho (B(\frac{1}{\sqrt{k}}))^p}{\lfloor m^{1/p}_k \rfloor^p }\cdot \sum_{i\in H_k}\sup_{\zeta,\phi}|M^{\zeta,\phi}_{i,2}(\lfloor m^{1/p}_k \rfloor,B(\frac{1}{\sqrt{k}}))|=O(\frac{\sqrt{\log k}}{\lfloor m^{1/2}_k \rfloor})=O(\sqrt{\log k}k^{-3/8})$$
since we have $m_k =  \Omega (k^{3/4})$.

%=========================================
\subsection{Proof of Theorem \ref{thm:minimizer}}
Recall that we assume $\cM^*_{\cF,\Phi}\subseteq\cF\times\Phi$ to be the set of minimizers of $L(\sD,f,\phi;\lambda)$. For a metric $dist(\cdot,\cdot)$ on the function class $\cF\times\Phi$, there exists a function $U(\cdot;\lambda):\bR\rightarrow\bR^{+}$ satisfying $\lim_{\varepsilon\rightarrow 0}U(\varepsilon;\lambda)\rightarrow 0$, such that for any $\varepsilon>0$
%, and any element $\xi\in\cF\times\Phi$,
$$\inf_{\xi \in\cF\times\Phi: ~\inf_{z\in\cM^*_{\cF,\Phi}}dist(\xi,z)\geq U(\varepsilon;\lambda)}|L(\sD,\xi;\lambda)-\min_{f\in\cF,\phi\in\Phi}L(\sD,f,\phi;\lambda)|\geq \varepsilon.$$

By Theorem \ref{thm:non-asymptotic bound}, 
$$\max_{f\in\cF,\phi\in\Phi}|\max_{\psi_k\in\Psi_k} L(S_{1:k},f,\phi,\psi_k;\lambda)-L(\sD,f,\phi;\lambda)|\leq \Gamma.$$

If we further denote 
$$(f^*_\lambda,\phi^*_\lambda)\in \argmin_{f\in\cF,\phi\in\Phi}L(\sD,f,\phi;\lambda) ,$$

it is not hard to see that
\begin{align*}
L(\sD,\hat{f}_\lambda,\hat{\phi}_\lambda;\lambda)-\min_{f\in\cF,\phi\in\Phi}L(\sD,f,\phi;\lambda)&= L(\sD,\hat{f}_\lambda,\hat{\phi}_\lambda;\lambda)-L(\sD,f^*_\lambda,\phi^*_\lambda;\lambda)\\
&\leq L(\sD,\hat{f}_\lambda,\hat{\phi}_\lambda;\lambda)- \max_{\psi_k\in\Psi_k} L(S_{1:k},f^*_\lambda,\phi^*_\lambda,\psi_k;\lambda)+\Gamma\\
&\leq  L(\sD,\hat{f}_\lambda,\hat{\phi}_\lambda;\lambda) -\max_{\psi_k\in\Psi_k} L(S_{1:k},\hat{f}_\lambda,\hat{\phi}_\lambda,\psi_k;\lambda)+\Gamma\\
&\leq 2\Gamma.
\end{align*}
Since $L(\sD,\hat{f}_\lambda,\hat{\phi}_\lambda;\lambda)-\min_{f\in\cF,\phi\in\Phi}L(\sD,f,\phi;\lambda)\geq 0$, by the above assumption, the result follows.

%=========================================
\subsection{Proof of Theorem \ref{thm:worstcase}}

Note that there are at most $\lfloor 1/p_l\rfloor$ elements in $\sD$ with $\mu$-probability at least $p_l$. As a result, with probability at least 
$$1-\frac{1}{p_l}\exp(-2\frac{(kp_l-m)^2}{k}),$$
over the randomness of the $k$ domains, all elements of $\sD$ with $\mu$-probability lower bounded by $p_l$ appears at least $m$ times in $k$ draws. Denote this event by $E$ and define $m=kp_l/2$. Under Assumption \ref{assumption:rep}, we know that for any domain $\cD_u\in\sD$, the $\delta$-neighborhood of $\cD_u$ under the notion of $\cH$-divergence contains some $\cD'_u$ that has $\mu$-probability lower bounded by $p_l$ and appears at least $kp_l/2$ times under event $E$. Thus, if $E$ occurs, then for all $f\in\cF$, $\phi\in\Phi$
$$\frac{kp_l}{2}\bP_{(x,y)\sim\cD'_u}(f(\phi(x))\neq y)\leq \sum_{i=1}^k \bP_{(x,y)\sim\cD_i}(f(\phi(x))\neq y)).$$

Since with probability at most $\sum_{i=1}^{k}4e^{-n_it^2}$ over the randomness of the $k$ domains, for a universal constant $c>0$
$$\frac{1}{k}\sum_{i=1}^k \bP_{(x,y)\sim\cD_i}(f(\phi(x))\neq y))\geq t+\frac{1}{k}\sum_{i=1}^{k}\frac{1}{n_i}\sum_{j=1}^{n_i}\bI\{f(\phi(x_{i,j}))\neq y_{i,j}\}+c\sqrt{\frac{\cV_{\Lambda}\log(n_i/\cV_{\Lambda})}{n_i}},$$
we have that with probability at least $1-\exp(-k^2p_l^2/2)/p_l-\sum_{i=1}^{k}4e^{-n_it^2}$
$$\bP_{(x,y)\sim\cD'_u}(f(\phi(x))\neq y)\leq\frac{2}{p_l} \Big(\hat{\beta}(f,\phi)+t+c\sqrt{\frac{\cV_{\Lambda}\log(n_i/\cV_{\Lambda})}{n_i}}\Big).$$
Using properties of $\cH$-divergence, we can then conclude that
$$\bP_{(x,y)\sim\cD_u}(f(\phi(x))\neq y)\leq \bP_{(x,y)\sim\cD'_u}(f(\phi(x))\neq y)+\delta.$$

\subsection{Proof of Theorem \ref{thm:existencemultiple}}

($\Rightarrow$) If there exists 
\begin{align*} 
f \in \text{Ker}(M_\phi) \,\, \text{s.t.~} \,\, \sum_{i=1}^k\bP_{x\sim\tilde{\cD}_i}(\Gamma(x)+f(x)\in M^{-}_\phi I_i(\psi_k))\leq\varepsilon
 \end{align*}
for some $\phi$, it follows that
 $$\sum_{i=1}^k\bP_{x\sim\tilde{\cD}_i}(\phi(x)+M_\phi f(x)\in  I_i(\psi_k))\leq\varepsilon.$$
Since we further have $f\in \text{Ker}(M_\phi)$
$$M_\phi f(x) = 0$$
for all $x$. Then,
 $$\sum_{i=1}^k\bP_{x\sim\tilde{\cD}_i}(\phi(x)\in  I_i(\psi_k))\leq\varepsilon.$$
 Since we have no ties, it is equivalent to say that
 $$\sup_{\psi_k\in\Psi_k}\sum_{i=1}^k\bP_{x\sim\tilde{\cD}_i^{\mathcal{X}}}(\pi_k\circ\psi_k(\phi(x))=i)\leq \varepsilon.$$

($\Leftarrow$) If instead $\sup_{\psi_k\in\Psi_k}\sum_{i=1}^k\bP_{x\sim\tilde{\cD}_i^{\mathcal{X}}}(\pi_k\circ\psi_k(\phi(x))=i)\leq \varepsilon,$ or equivalently

 $$\sum_{i=1}^k\bP_{x\sim\tilde{\cD}_i}(\phi(x)\in  I_i(\psi_k))\leq\varepsilon,$$
then, 
 $$\sum_{i=1}^k\bP_{x\sim\tilde{\cD}_i}(M_\phi\Gamma(x)\in  I_i(\psi_k))\leq\varepsilon.$$
This leads to 
\begin{align*} 
\sum_{i=1}^k\bP_{x\sim\tilde{\cD}_i}(\Gamma(x)\in M^{-}_\phi I_i(\psi_k)+Ker(M_\phi))\leq\varepsilon,
 \end{align*}where $M^{-}_\phi$ is the M-P inverse of $M_\phi$.

Consider $f(x)=M^{-}_\phi M_\phi\Gamma(x)-\Gamma(x)$. It is easy to see that for $z\in\bR^s$, the pre-image of $z$ under $M_\phi$ in $\bR^m$ is $M^{-}_\phi z+Ker(M_\phi)$. Thus, if 
$$M_\phi \Gamma(x)=z,$$
we have
$$\Gamma(x)+f(x)=M^{-}_\phi z.$$
Now notice  that for $\Gamma(x)\in  M_\phi^{-}z+Ker(M_\phi)$, $\Gamma(x)+f(x)=M_\phi^{-}z.$
Consequently, $f$ maps  pre-images of $z$ to $M^-_\phi z$, thus, if 
 $$\sum_{i=1}^k\bP_{x\sim\tilde{\cD}_i}(\phi(x)\in  I_i(\psi_k))\leq\varepsilon,$$
we have
$$ \sum_{i=1}^k\bP_{x\sim\tilde{\cD}_i}(\Gamma(x)+f(x)\in M^{-}_\phi I_i(\psi_k))\leq\varepsilon.$$

\section{Details of Experiments}

This section includes details of the network architecture, specific data generation methods, and additional experiments not mentioned in the paper. 
%{\color{red} PS: We did not refer to supplement including additional experiments. I am iin favor of deleting this part for Neurips, but including in arxiv version.}

\subsection{Architecture}

For all experiments, we train our model with batch size $64$ for $100$ epochs and then take the test accuracy when the total loss has stabilized. For computation, each experiment is run over a machine with Intel "Cascade Lake" CPU Core with a V100 GPU.

The discriminator and predictor classes were chosen to be identical traditional feed-forward MLPs, along with the encoder class for synthetic data. The number and width of the hidden layers depend on the dataset and are specified in the sections below. Since colored MNIST and PACS datasets are image data, the encoder was chosen to be a convolutional neural network.

For each dataset setting, we optimize our algorithm through searching over the tuning parameter $\lambda$ for adversarial loss, along with the learning rate; we find best results with a learning rate of $0.001$. In each setting, we then fix the best reported $\lambda$ and report the average test accuracy taken over multiple runs.

Note that in every setting we run, the validation and training data are randomly split with size proportions $20\%/80\%$ respectively among the $k$ training studies. We denote $k$-Domain to represent a setting with $k$ training studies. In the synthetic data, each domain, including the unseen domain, had $5000$ samples. In the colored MNIST data, each domain, including the unseen domain, had $10,000$ samples. In the binary version of PACS data, each of the $4$ domains had $384,540,803,1493$ samples respectively. In the following sections, we mention the specific details for each dataset that have been omitted from the main article. 

\subsection{Synthetic Data}

Recall that the dimension of the input covariates for the synthetic data was $30$. We chose the encoded representations $Z=\phi(X)$ to have dimension $10$. The networks for the classifier and discriminator have $6$ hidden layers, each containing $10$ nodes. The base rates $b_i$ were taken to be the same across studies and equals $0.7$ for label $1$. For the covariate distributions, each mean vector $\mu_k$ lies in dimension $30$, where each entry was drawn randomly from $[-3, 3]$. The covariance matrices $\Sigma_k$ are of dimension $30\times 30$---these are obtained by first {\color{red}
defining a matrix $\sigma$ of the same dimensions with each value drawn randomly from $[1, -1]$, and then setting $\Sigma = \sigma\times\sigma^T$.} {\color{red} Does not make sense. Do we mean $\sigma$ is a vector in $\mathbb{R}^{30}$?}

\subsubsection{Classification Rules}

\textbf{Classification rule is linear with one product interaction} referenced in Table 1 (a):

We first fix $\hat w$ to be a vector of size $20$ with each value sampled uniformly between $[0.25, 2]$. Also fix $\lambda$ by choosing a value uniformly among $[0.25, 1]$.

For a datapoint $x_j\in \mathbb R^{30}$ from domain $\mathcal D_i$ and subset $\mathcal A \in \mathbb R^{20}$ which represents the common covariates, we have the following classification rule: 

\[f_{\mathrm{inv}}(x_{j,\mathcal{A}}, \epsilon_{i, \mathcal{A}}) = w(\epsilon_{i, \mathcal{A}})^T x_{j,\mathcal{A}}+\lambda x_{j,a\in\mathcal{A}} x_{j,b\in\mathcal{A}}\]

Above, $a$ and $b$ refer to two randomly chosen common covariates and $w$ is a vector of size $20$ (the number of common covariates).
To construct $w$ for domain $\mathcal D_i$, $\hat w$ is perturbed slightly, so that for each entry $w_a \in w$ that is associated with a common covariate $a\in \mathcal A$, let $\epsilon_{i, a}$ is drawn uniformly at random from $[-0.1, 0.1]$ and  $w_a = \hat{w_a} + \epsilon_{i, a}$. This builds in some error in the invariant function.

For $f_i$, the study-specific classification rule for domain $\mathcal D_i$, we similarly have the following:

\[f_{\mathrm{i}}(x_{j,\mathcal{A}^c}, \epsilon_{i, \mathcal{A}^c}) = w'(\epsilon_{i, \mathcal{A}^c})^T x_{j,\mathcal{A}^c}+\lambda x_{j,a\in\mathcal{A}^c} x_{j,b\in\mathcal{A}^c}.\]

% For each w_j that is associated with a study-specific covariate, the final w*_j will be uniformly from [w_j+2, w_j+2].

To construct study-specific $w'$ for domain $\mathcal D_i$, $\hat w$ is once again perturbed but to a larger extent, so that for each entry $w_a \in w$ that is associated with a study-specific covariate $b\in \mathcal A^c$,  $\epsilon_{i, b}$ is drawn uniformly at random from $[-2, 2]$ and $w_b = \hat{w_b} + \epsilon_{i, b}$.

\textbf{Classification rule as the logical OR of two linear functions} referenced in Table 1 (b):
We first fix $\hat{w_1}, \hat{w_2}, \hat{w_3}$ as $3$ vectors of size $20$ with entries of each sampled uniformly between $[0.25, 2]$.

{\color{red} For invariant classification rule $f_{\mathrm{inv}}$, for each entry $w_{1,a} \in w_1$ that is associated with a common covariate $a\in \mathcal A$, let $\epsilon_{i, a}$ be drawn uniformly at random from $[-0.1, 0.1]$. The final $w_{1,a} = \hat{w_{1,a}} + \epsilon_{i, a}$. The same is true for $w_2$.

Let $p_1 = \mathrm{sigmoid}(w_1^T x_{j,\mathcal{A}})$ and let $p_2 = \mathrm{sigmoid}(w_2^T x_{j,\mathcal{A}})$). Then $y_1 = 1$ with probability $p_1$ and $0$ otherwise, and $y_2 = 1$ with probability $p_2$ and $0$ otherwise. The final output is $y = y_1 \mathrm{OR} y_2$.

For study-specific classification rule $f_{\mathrm{i}}$, we make the study-specific signal "easier" to learn than g:

\[f_i(x_{j,{\mathcal{A}^c}}) = w_3^T x_{j,{\mathcal{A}^c}}\]

For each entry $w_{3,b} \in w_1$ that is associated with a study-specific covariate $b\in \mathcal A^c$, let $\epsilon_{i, b}$ be drawn uniformly at random from $[-2, 2]$. The final $w_{3,b} = \hat{w_{3,b}} + \epsilon_{i, b}$.} {\color{red} PS: This still needs some cleaning, but I am crashing today.} 

\subsection{Colored MNIST}

The input size for an image from the MNIST dataset is $3\times 28\times 28$, we chose the representation space dimension to be  $50$. The networks for the classifier and discriminator have $6$ hidden layers, each $200$ nodes wide.

\subsubsection{Settings}

%For all of our colored MNIST settings, we follow similar dataset generation to that of IRM \cite{arjovsky2019invariant}. In the case of \textbf{2-Domain settings} of $A\%$-shape $B\%$-color. We do the following procedure on the regular MNIST dataset: let $\hat y=1$ for digits $5-9$ and $\hat y = 0$ otherwise. With $A\%$ probability, let $y = \hat y$, and otherwise let $y = 1-\hat y$, where $y$ is now the final label. For domain 1, if an image has label $1$, then color the digit green with $B\%$ probability and red otherwise; if an image has label $0$, then color the digit red with $B\%$ probability and green otherwise. For domain 2, if an image has label $1$, then color the digit red with $B\%$ probability and green otherwise; if an image has label $0$, then color the digit green with $B\%$ probability and red otherwise.

\textbf{6-Domain unequal color setting} referenced in Table 4 Row 3: There was a $100\%$ shape-label correlation across all of the studies. Study 1 had $80\%$ red-green color correlation (where red $80\%$ correlated with label $0$ and green $80\%$ correlated with label $1$), Study 2 had 60\% red-green color-label correlation (where red $60\%$ correlated with label $0$ and green $60\%$ correlated with label $1$), and Study 3 had 40\% red-green color correlation (where red $40\%$ correlated with label $0$ and green $40\%$ correlated with label $1$). Study 4 had $70\%$ blue-yellow color-label correlation (where blue $70\%$ correlated with label $0$ and yellow $70\%$ correlated with label $1$). Study 5 label 1 images were red with $10\%$ probability, green with $10\%$ probability, and yellow with $80\%$ probability; label 0 images were red with $70\%$ probability, green with $20\%$ probability, and yellow with $10\%$ probability. Study 6 had $80\%$ red-blue color-label correlation (where red $80\%$ correlated with label $0$ and blue $80\%$ correlated with label $1$). The test study had completely white digits.

\textbf{3-Domain setting} referenced in Table 2 Column 1: The dataset used to directly compare to the above 6-Domain setting had Studies 1, 3, and 5 from the above description as the training datasets. The test study was completely identical. 

\subsection{PACS}

The input size for an image from the PACS dataset is $3\times 64\times 64$, with the representation space of dimension $1000$. The networks for the classifier and discriminator have $4$ hidden layers, each containing $1000$ nodes. 
%(The number of hidden layers decreases from $6$ due to computation power limits from a large input size.)

\subsection{Introduction of Decoder}
Note that all of our experiments so far excluded the decoder from the LAFTR architecture \cite{madras2018learning}. The inquisitive reader may wonder whether including the decoder improves or harms the performance. We performed extensive experiments to investigate this question---some of the experimental results are summarized below. In the process, we examined the reconstruction images to determine whether the study ID was being effectively hidden.

% the differences that would occur if we had instead included the decoder. We study thi
%Based on the presence of a decoder in the LAFTR model \cite{madras2018learning}, along with the encoder, discriminator, and classifier, we explore whether a decoder improves or harms performance. We also use the decoder to determine whether the study ID is effectively being hidden through examination of the reconstruction images.

In the subsequent experiments, we consider the following loss function, which contains an additional term corresponding to the reconstruction loss $L_{Decoder}$---in practice, this is implemented using the binary cross entropy. 

\[\mathcal{L} := L_{Classifier} + \beta L_{Decoder} + \lambda L_{Adversary}\]

\subsubsection{Reconstruction}
Consider an experimental setting involving a colored MNIST data of the form $100\%$ shape-$90\%$-color, with a test dataset of entirely purple images. Figures \ref{fig:colorvalid} and \ref{fig:colortest} display a subset of the decoder reconstruction images and ground truth images . 
It is evident that the color feature is not preserved in the reconstruction -- several digits have mixtures of red and green digits, while others have flipped colors completely. This may indicate that the encoder is no longer storing color information in the representations $Z$, which allows the adversary to have difficulty determining which domain an image belongs to. This setting had validation accuracy of $98.0\%$ and test accuracy of $97.6\%$.

%These images are from experimental setting of $100\%$-shape and $90\%$-color, with a test dataset of entirely purple images. Here, it is evident that the color feature is not preserved in the decoder reconstruction images -- several images have mixed red and green, while others completely flipped colors. This may indicate that the encoder is no longer storing color information in $Z$, which allows the adversary to have difficulty determining which domain an image belongs to. This setting had validation accuracy of $98.0\%$ and test accuracy of $97.6\%$.

\begin{figure} [H]
  \centering
  \includegraphics[width=9cm]{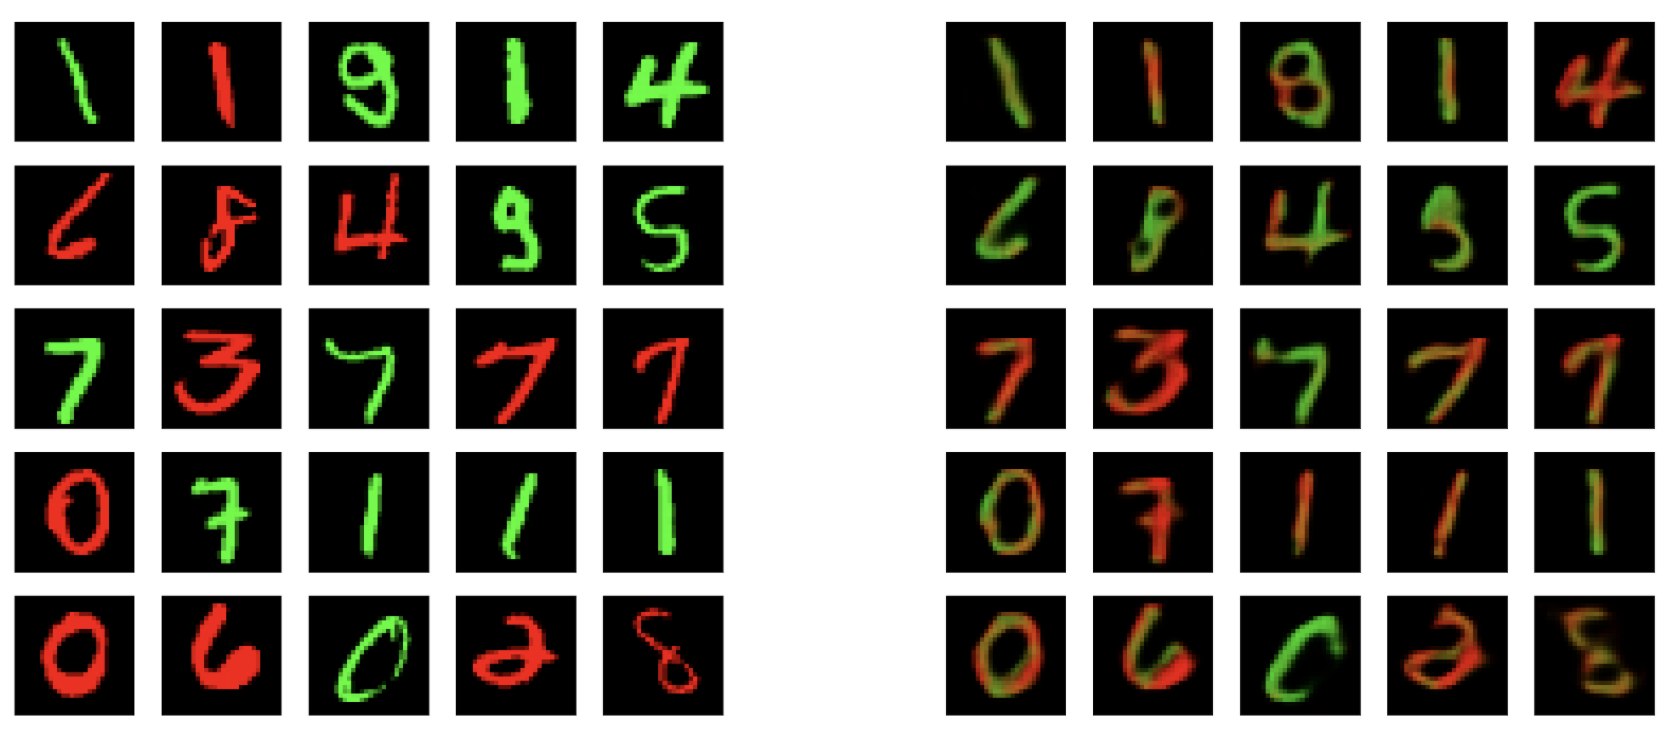}
  \caption{Ground truth images compared to decoder based reconstruction images from validation data of colored MNIST on a $100\%$shape-$90\%$color setting; the test dataset contained purple images.}
  \label{fig:colorvalid}
\end{figure}

%\begin{figure} [H]
% \centering
 % \includegraphics[width=9cm]{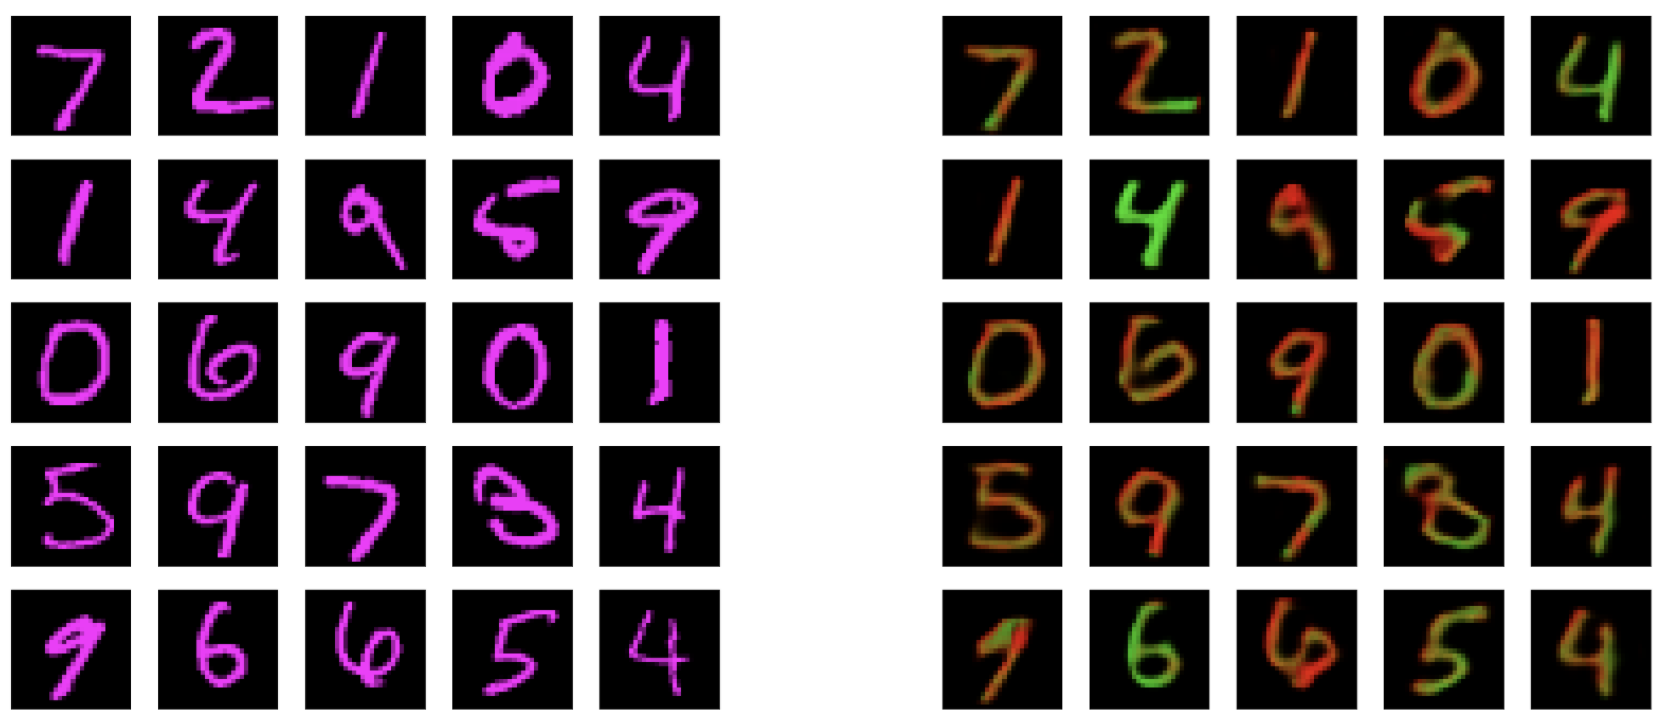}
 % \caption{Same setting as Figure \ref{fig:colorvalid}, but comGround truth images compared to decoder reconstruction images from test data of colored MNIST on setting of $100\%$-shape and $90\%$-color, with a test dataset of entirely purple images.}
 % \label{fig:colortest}
%\end{figure}

\subsubsection{Comparisons}

We next compare the performance of the proposed algorithm with and without the decoderon variety of colored MNIST data settings. Table \ref{colordecoder} shows that the test accuracy remains similar across the settings. 
% we see the presence of the decoder has similar test accuracy than without the decoder.

\textcolor{red}{Note that the experiment results with a decoder are only over a single trial. Running over multiple trials now.}

\begin{table}[H]
  \caption{Decoder versus no decoder comparison of test accuracy on various colored MNIST settings. $k$ refers to the number of training studies.}
  \label{colordecoder}
  \centering
  \begin{tabular}{llllll}
    \toprule
    & Setting & Target & $k$ & No Decoder & Decoder \\
    \midrule
    1. & $100\%$-shape $90\%$-color & purple & 2 & 97.5\% & 97.6\% \\
    \midrule
    2. & $75\%$-shape $80\%$-color & red-green & 2 & 69.7\% & 72.9\% \\
    \midrule
    3. & $100\%$-shape unequal color correlation & white & 6 & 97.7\% & 98.1\% \\
    \bottomrule
  \end{tabular}
\end{table}

\subsubsection{Trivial Case}
A  natural question that may arise is the followin: is there any intuitive reason for including (or not including) the decoder. Here, we discuss this issue by demonstrating a particular phenomenon that occurs in some settings in the absence of the decoder. Consider a colored MNIST data setting of $75\%$-shape $80\%$-color. When the coefficients for reconstruction and fairness losses are too low, for example $\beta = \lambda = 0.05$, we found that RVR (that is, without a decoder) obtains a validation accuracy of $81.0\%$ and a test accuracy of $56.7\%$. Notice that the validation accuracy here is close to the color-label correlation magnitude and, simultaneously, such a low test accuracy indicates that perhaps the encoder is not learning the invariant signal which is shape, but instead learning color and study ID.

To investigate this further, we performed a PCA of the encoded representations $Z=\phi(X)$. Figure \ref{fig:clustering} depicts the first two principal components and we observe that both color and study ID are grouped separately. We conjecture that  this implies the following: on the input latent representation $Z$, the classifier would only have to record the study ID and color, based on which cluster the input belongs to, in order to determine the label with $80\%$ accuracy on the validation data. Naturally, if this were true, this method would not perform well on the test dataset since there is no color correlation with label there. Studying this phenomenon further is a promising direction of future research, and is expected to yield a better understanding of settings where our proposed algorithm should work well. Despite such settings where the absence of the decoder hurts, we observe extremely good prediction performance in a host of other settings without the decoder. Mostly, even a coarse optimization of the hyperparameters sufficed to ensure that this critical situation would not arise in the absence of the decoder. 

\begin{figure} [H]
  \centering
  \includegraphics[width=13cm]{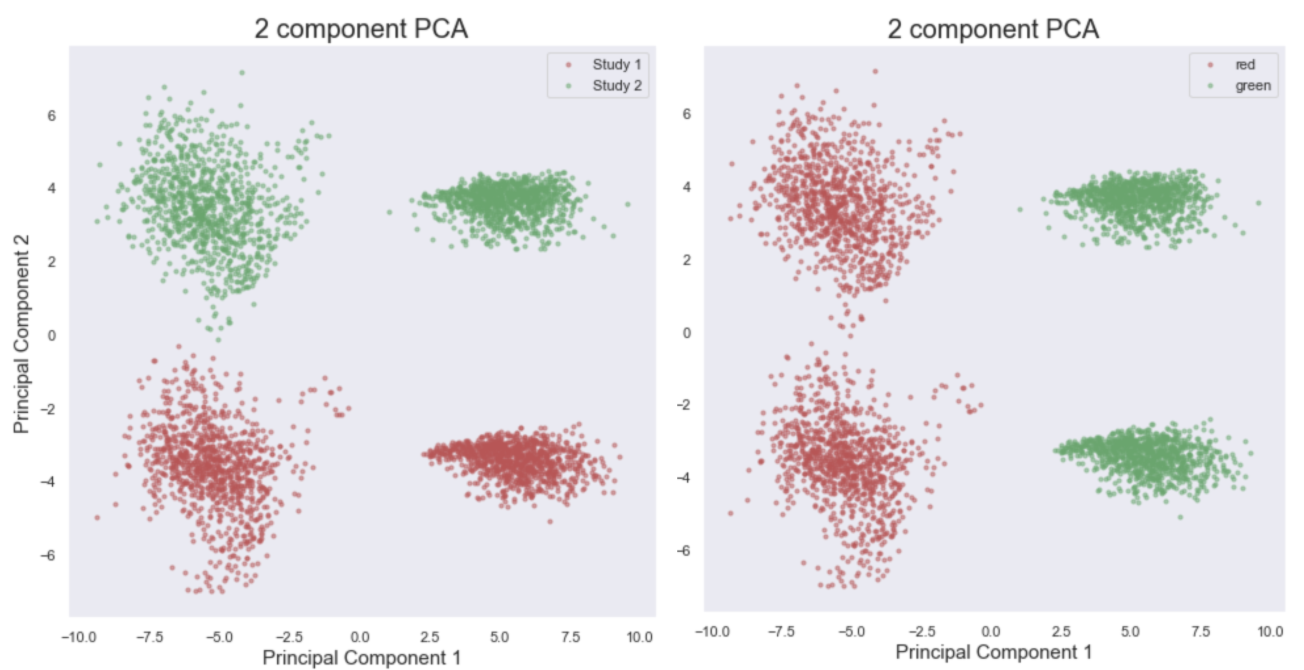}
  \caption{Principal components of the encoded representations $Z$ in validation data for $75\%$-shape $80\%$-color setting with validation accuracy $81.0\%$ and test accuracy $56.7\%$; the test data contained red and green digits with no correlation. The color on the left plot is based on study ID whereas that on the right plot is based on digit color.}
  \label{fig:clustering}
\end{figure}
